# Supplementary material for: A Structural and Algorithmic Study of Stable Matching Lattices of "Nearby" Instances, with Applications
Source: arXiv:1804.05537 source file (2022-08-15)
Supplement: Supplementary file 1 [file ack.tex]

\section{Acknowledgement}
\label{sec.ack}

We wish to thank Professor Richard Stanley and an anonymous reviewer for helping us confirm the status of Theorem \ref{thm:generalization}.
