# Supplementary material for: A Structural and Algorithmic Study of Stable Matching Lattices of "Nearby" Instances, with Applications
Source: arXiv:1804.05537 source file (2022-08-15)
Supplement: Supplementary file 8 [file overview.tex]

\subsection{Overview of structural and algorithmic ideas}
\label{sec.overview}
